# Supplementary material for: What Evidence We Would Miss If We Do Not Use Grey Literature?
Source: arXiv:2107.05792 source file (2021-08-17)
Supplement: Supplementary file 1 [file appendixA.tex]

\appendix{Appendix - Investigated Studies}\label{appendix-mlr-studies-investigated}

%\noindent{\large\bfseries Included Secondary Studies References\par}
%\subsection{References}

\nocitesec{*}
%\bibliographystylesec{elsarticle-num}
\bibliographystylesec{ACM-Reference-Format}
\bibliographysec{secondaryStudiesNotIncluded}
